# Supplementary material for: Planar Object Tracking via Weighted Optical Flow
Source: arXiv:2301.10057 source file (2023-01-24)

# POT-210 all

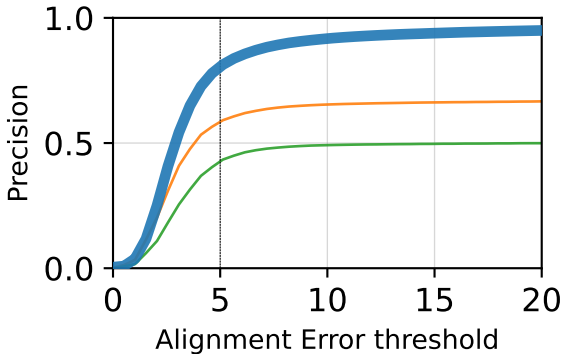

# POT-210 scale

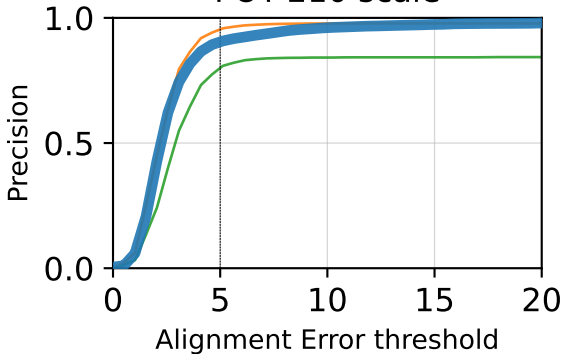

# POT-210 rotation

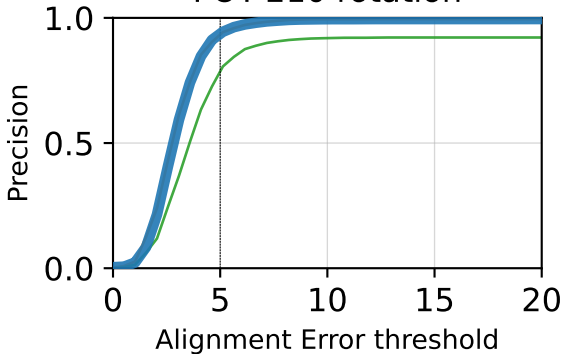

POT-210 perspective

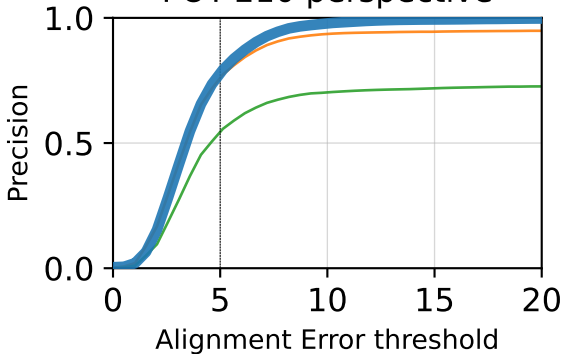

POT-210 blur

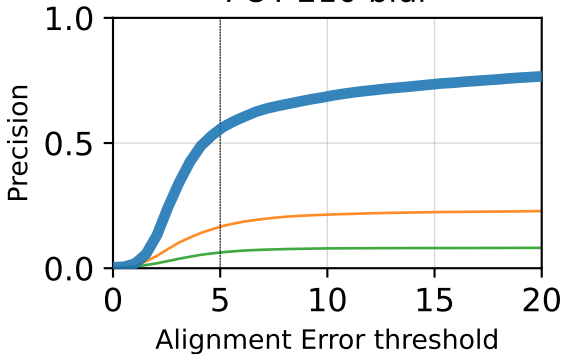

POT-210 occlusion

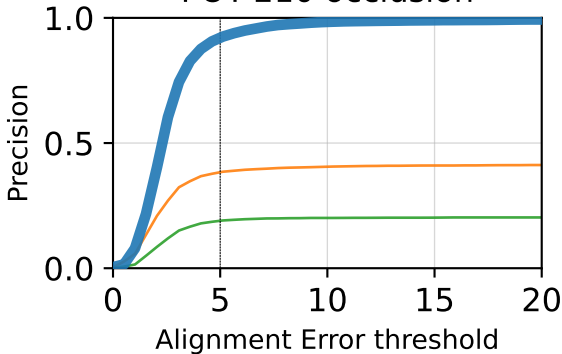

POT-210 out-of-view

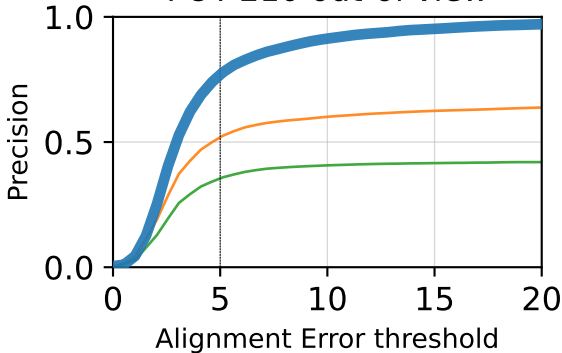

POT-210 unconstrained

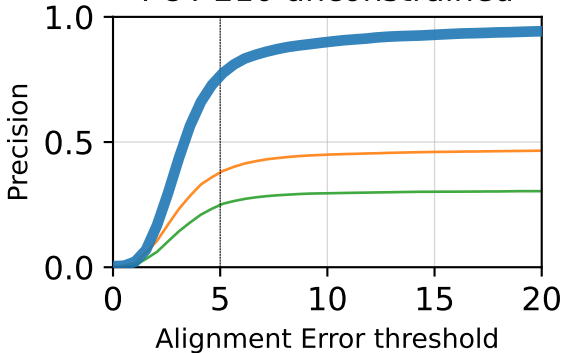

Supplement: Supplementary file 3 [file POT210_direct_merged_AE_roc.pdf]
