# Supplementary material for: Planar Object Tracking via Weighted Optical Flow
Source: arXiv:2301.10057 source file (2023-01-24)

**all**

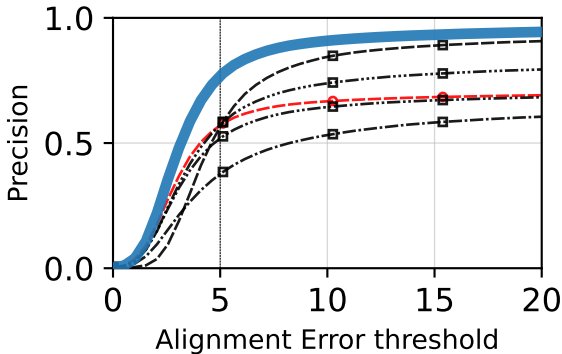

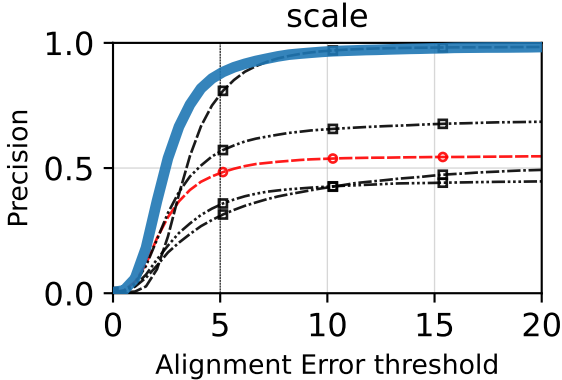

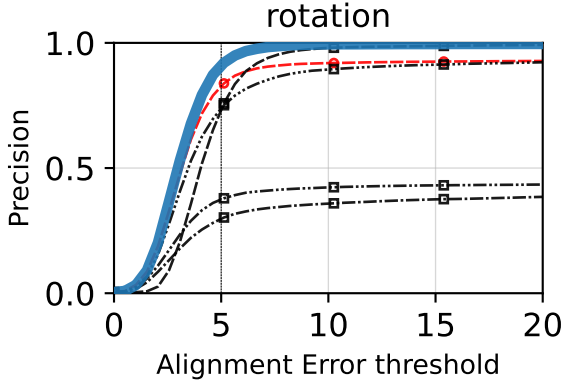

perspective

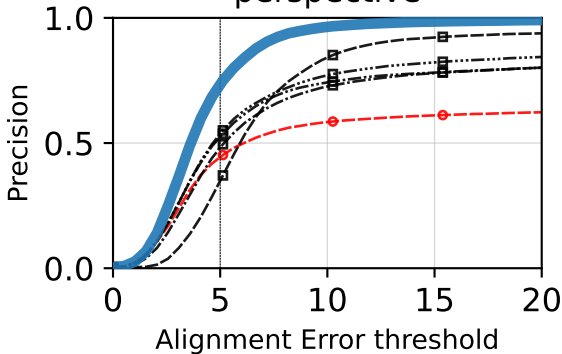

blur

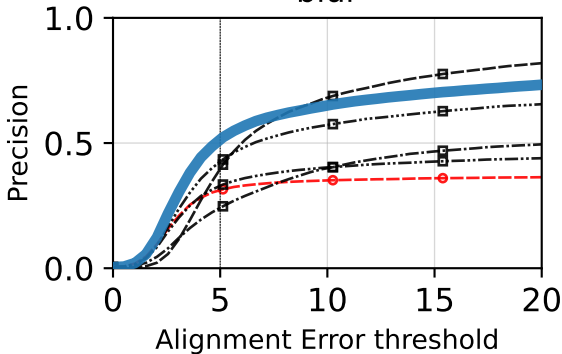

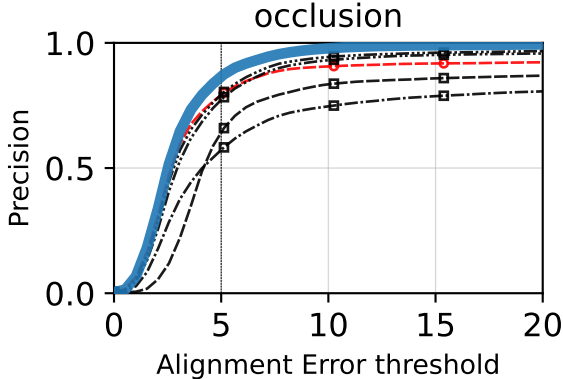

out-of-view

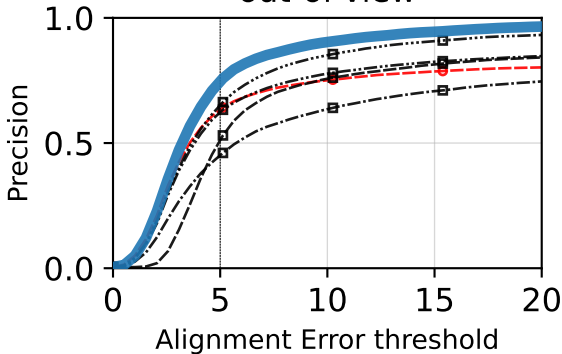

unconstrained

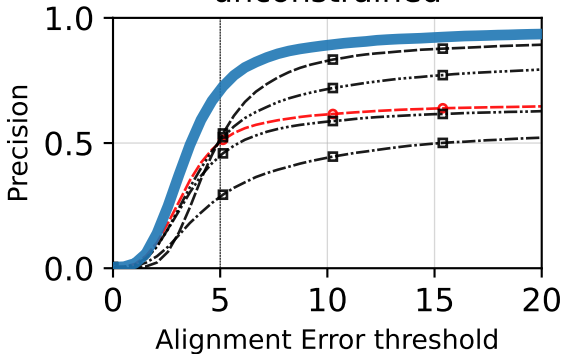

Supplement: Supplementary file 5 [file POT280_merged_AE_roc.pdf]
